# Supplementary material for: Scene-LLM: Extending Language Model for 3D Visual Understanding and Reasoning
Source: arXiv:2403.11401 source file (2024-03-22)
Supplement: Supplementary file 1 [file tab_0_result_qa.tex]

\begin{table*}[!t]
\centering
\small
\caption{Answer accuracy on ScanQA using object proposals from Mask3D. Each entry  denotes ``val'' / ``test w/ object'' / ``test w/o object''.}\label{tab:scanqa}
\begin{tabular}{lccccccc}
\toprule
Method & \multicolumn{1}{c}{EM@1} & \multicolumn{1}{c}{EM@10} & \multicolumn{1}{c}{BLEU-1} & \multicolumn{1}{c}{BLEU-4} & \multicolumn{1}{c}{ROUGE} & \multicolumn{1}{c}{METEOR} & \multicolumn{1}{c}{CIDEr}\\
\midrule
Image+MCAN \cite{scanqa} & 22.3 / 20.8 & 53.1 / 51.2 & 14.3 / 9.7 & 31.3 / 29.2 & 12.1 / 11.5 & 60.4 / 55.6 \\
ScanRefer+MCAN \cite{scanqa} & 20.6 / 19.0 & 52.4 / 49.7 & 7.5 / 7.8 & 30.7 / 28.6 & 12.0 / 11.4 & 57.4 / 53.4 \\
ScanQA \cite{scanqa} & 23.5 / 20.9 & 56.5 / \textbf{54.1} & 12.0 / 10.8 & 34.3 / 31.1 & 13.6 / 12.6 & 67.3 / 60.2 \\
3D-LLM & \textbf{27.0} / \textbf{23.0} & \textbf{57.9} / 53.5 & \textbf{16.0} / \textbf{11.9} & \textbf{38.6} / \textbf{32.8} & \textbf{15.2} / \textbf{12.9} & \textbf{76.6} / \textbf{62.6} \\
3D-Vista & \textbf{27.0} / \textbf{23.0} & \textbf{57.9} / 53.5 & \textbf{16.0} / \textbf{11.9} & \textbf{38.6} / \textbf{32.8} & \textbf{15.2} / \textbf{12.9} & \textbf{76.6} / \textbf{62.6} \\
\bottomrule
\end{tabular}
\end{table*}

\begin{table*}[!h]
\begin{minipage}[t]{0.60\textwidth}
\centering
\small
\caption{Answer accuracy on SQA3D using object proposals from Mask3D. Pre-training improves the results of most question types.}\label{tab:sqa3d}
\resizebox{\linewidth}{!}{
\begin{tabular}{lccccccc}
\toprule
\multirow{2}{*}{Method} & \multicolumn{6}{c}{Test set} & \multirow{2}{*}{Avg.} \\ 
\cline{2-7}
& What & Is & How & Can & Which & Other & \\ 
\hline
GPT-3 \cite{sqa3d} & \textbf{39.7} & 46.0 & 40.5 & 45.6 & 36.1 & 38.4 & 41.0 \\ 
ClipBERT \cite{sqa3d} & 30.2 & 60.1 & 38.7 & 63.3 & 42.5 & 42.7 & 43.3 \\
SQA3D(w/o s) \cite{sqa3d} & 28.6 & 65.0 & 47.3 & 66.3 & 43.9 & 42.9 & 45.3 \\
SQA3D \cite{sqa3d} & 31.6 & 63.8 & 46.0 & 69.5 & 43.9 & 45.3 & 46.6 \\
\midrule
\model (scratch) & 32.1 & 62.9 & \textbf{47.7} & 60.7 & 45.9 & \textbf{48.9} & 46.7 \\ 
\model & 34.8 & \textbf{63.3} & 45.4 & \textbf{69.8} & \textbf{47.2} & 48.1 & \textbf{48.5} \\ 
$\Delta$ & \inc{2.7} & \inc{0.4} & \dec{2.3} & \inc{9.1} & \inc{1.3} & \dec{0.8} & \inc{1.8} \\ 
\bottomrule
\end{tabular}

}
\end{minipage}
\hfill
\begin{minipage}[t]{0.38\textwidth}
\centering
\captionof{figure}{\label{fig:data_efficiency} The performance of finetuning \model using various amounts of training data.} 
\includegraphics[width=\linewidth]{limit.pdf}
\end{minipage}
\end{table*}
